# Supplementary material for: Systematic Search for FFPs in KMTNet Full-Frame Images. I. Photometry Pipeline
Source: arXiv:2503.24097 source file (2025-06-17)
Supplement: Supplementary file 1 [file Appendix.tex]

\section{Re-conduction of KMTNet events}\label{sec:appendix}

\section{Re-conduction of OGLE events}\label{sec:appendix}

\section{New microlensing event candidates}\label{sec:appendix}

%\begin{figure*}[ht!]
%    \centering
%    \includegraphics[scale=0.4]{figures/newevent.png}
%    \caption{New event. }
%    \label{fig:revisewin}
%\end{figure*}
